# Supplementary material for: Unsupervised Story Discovery from Continuous News Streams via Scalable Thematic Embedding
Source: arXiv:2304.04099 source file (2023-05-04)
Supplement: Supplementary file 1 [file 8.Appendix.tex]

\section{Supplemental Material}
\subsection{Pseudo-code of \algname{}}
\label{apd:pseudocode}
%For every sliding window of an article stream, \algname{} get sentence representations of new articles with a pretrained sentence encoder and derive initial article representation (Lines 1$-$4). When there are no existing stories (e.g., in case of the first window), the initial seed stories are found from the new articles (Lines 5$-$6). Then, for each unassigned article in the window, \algname{} derives representations of the article and existing stories and calculates the maximum confidence score of the article to be added to one of existing stories. Here, the pane-based story summary (PSS) is used to facilitate the computation instead of accessing all previous articles. If the score is above the threshold, the article is assigned to the corresponding story, and the corresponding PSS is updated (Lines 7$-$12 and Figure \ref{fig:method_overview}a). Those which are not confident enough to be added to existing stories are used to find novel seed stories (Line 13 and Figure \ref{fig:method_overview}b). The following sections explain the main components in \algname{}, the novel seed stories discovery, the confidence-based story assignment, and the story summary maintenance, in detail.
